# Supplementary material for: Non-Wellfounded and Cyclic Proofs for LTL: A Syntactic Correspondence with Linear Nested Sequents
Source: arXiv:2606.03413 source file (2026-10-05)
Supplement: Supplementary file 1 [file sec-appendix.tex]

We provide the proofs of soundness and completeness of the non-wellfounded calculus $\calci$. For soundness, we argue by contradiction: we suppose that an invalid LNS $\lnsg$ has a non-wellfounded proof in $\calci$ and show how to obtain from this assumption an infinite, strictly decreasing sequence of natural numbers, thus yielding a contradiction. To that end, let $\lnsg$ be an LNS. A \emph{progress measure} for $\lnsg$ is a map $\mu$ which assigns to each trace value $\bracket{A \until B, j}$ of $\lnsg$ a natural number.

\begin{customthm}{\ref{thm:soundness}}[Soundness of $\calci$]
If $\calci \proves \lnsg$, then $\lnsg$ is valid.
\end{customthm}
\begin{proof}
    Let $\pi$ be a non-wellfounded proof of $\lnsg$ and suppose, for contradiction, that $\lnsg$ is invalid. Then, there exists a state sequence $\model$ such that $\model, 0 \not \sat \lnsg$. We will inductively define an infinite path of LNSs $\set{\lnsg_i}_{i \in \mathbb{N}}$ through $\pi$ and an infinite sequence of progress measures $\set{\mu_i}_{i \in \mathbb{N}}$ such that for all $i \in \mathbb{N}$ the following hold:
    \begin{enumerate}
        \item[$(1)$]$\model, 0 \not \sat \lnsg_i$;
        \item[$(2)$] $\mu_i$ is a progress measure for $\lnsg_i$;
        \item[$(3)$] for every trace value $\bracket{A \until B,j}$ of $\lnsg_i$ the following hold:
        \begin{enumerate}
            \item $\mu_i(\bracket{A \until B,j})$ is the least natural number $k$ such that $\model, j+k \sat B$ and $\model, j+k' \sat A$ for each $0 \leq k' < k$;
            \item if $(\bracket{A \until B,j}, \bracket{A \until B,j})$ is a trace pair for $(\lnsg_{i-1}, \lnsg_{i})$, then $\mu_{i}(\bracket{A \until B,j}) \leq \mu_{i-1}(\bracket{A \until B,j})$;
            \item if $(\bracket{A \until B,j}, \bracket{A \until B,j+1})$ is a trace pair for $(\lnsg_{i-1}, \lnsg_{i})$, then $\mu_{i}(\bracket{A \until B,j+1}) < \mu_{i-1}(\bracket{A \until B,j})$.
        \end{enumerate}
    \end{enumerate}
We now define $\set{\lnsg_i}_{i \in \mathbb{N}}$ and $\set{\mu_i}_{i \in \mathbb{N}}$. First, let $\lnsg_0 := \lnsg$. Since $\model, 0 \not \sat \lnsg$, we have $\model, j \sat A \until B$ for each trace value $\bracket{A \until B, j}$ of $\lnsg$. Therefore, for any trace value $\bracket{A \until B, j}$ of $\lnsg$, there exists a natural number $k$ such that (i) $\model, j + k \sat B$, and (ii) $\model, j + k' \sat A$ for each $0 \leq k' < k$. Hence let $\mu_0$ be the map that assigns to each trace value $\bracket{A \until B, j}$ of $\lnsg$ the least natural number $k$ such that (i) and (ii) hold. One can readily verify that conditions (1)--(3) are satisfied.

Suppose we have defined $\lnsg_i$ and $\mu_i$ and they satisfy (1)--(3). We define $\lnsg_{i+1}$ and $\mu_{i+1}$ by using a case distinction based on the rule $\mathsf{r}$ with conclusion $\lnsg_i$ in $\pi$. Note that $\mathsf{r}$ cannot be an initial rule, since $\model, 0 \not \sat \lnsg_i$ by (1). We show the case for $\untilli$; the other cases are argued similarly. Suppose $\lnsg_i$ is the conclusion of an instance of $\untilli$, as shown below.
    \begin{center}
\begin{tabular}{c}
\AxiomC{$\overbrace{\lnsg \sep \Gamma, B \sar \Delta \sep \Sigma \sar \Pi \sep \lnsh}^{\lnsg'}$}
\AxiomC{$\overbrace{\lnsg \sep \Gamma, A \sar \Delta \sep \Sigma, A \until B  \sar \Pi \sep \lnsh}^{\lnsg''}$}
\RightLabel{$\untilli$}
\BinaryInfC{$\underbrace{\lnsg \sep \Gamma, A \until B \sar \Delta \sep \Sigma \sar \Pi \sep \lnsh}_{\lnsg_i}$}
\DisplayProof
\end{tabular}
\end{center}

Suppose $\Gamma, A \until B \sar \Delta$ is the $j$-component of $\lnsg_i$ and the principal formula forms the trace value $\bracket{A \until B, j}$ of $\lnsg_i$. We now make a case distinction on if $\mu_i(\bracket{A \until B, j}) = 0$ or $\mu_i(\bracket{A \until B, j}) > 0$.

If $\mu_i(\bracket{A \until B, j}) = 0$, then $\model, j \sat B$. Hence, let $\lnsg_{i+1} := \lnsg'$ and observe that $\model, 0 \not \sat \lnsg_{i+1}$. If $B=C \until D$ for some formulae $C,D$, then let $\mu_{i+1}(\bracket{B,j})$ be the least natural number $k$ such that $\model, j+k \sat D$ and $\model, j+k' \sat C$ for each $0 \leq k' < k$. For any other trace value $\bracket{C \until D, l}$ of $\lnsg_{i+1}$, $(\bracket{C \until D, l}, \bracket{C \until D, l})$ is a trace pair for $(\lnsg_i, \lnsg_{i+1})$. Therefore, let $\mu_{i+1}(\bracket{C \until D, l}) := \mu_i(\bracket{C \until D, l})$. Note that (1)--(3) are satisfied.

If $\mu_i(\bracket{A \until B, j}) > 0$, then observe that $\model, j \sat A$ and $\model, j+1 \sat A \until B$ by (3)-(a). Hence, let $\lnsg_{i+1} := \lnsg''$ and note that $\model, 0 \not \sat \lnsg_{i+1}$. If $A=C \until D$ for some formulae $C,D$, then let $\mu_{i+1}(\bracket{A,j})$ be the least natural number $k$ which satisfies that $\model, j+k \sat D$ and $\model, j+k' \sat C$ for each $0 \leq k' < k$. Furthermore, let $\mu_{i+1}(\bracket{A \until B, j+1}) := \mu_i(\bracket{A \until B, j}) - 1$. For any other trace value $\bracket{E \until F, l}$ of $\lnsg_{i+1}$, $(\bracket{E \until F, l}, \bracket{E \until F, l})$ is a trace pair for $(\lnsg_i, \lnsg_{i+1})$. Therefore, let $\mu_{i+1}(\bracket{E \until F, l}) := \mu_i(\bracket{E \until F, l})$. Note that (1)--(3) are satisfied. This concludes the construction of $\set{\lnsg_i}_{i \in \mathbb{N}}$ and of $\set{\mu_i}_{i \in \mathbb{N}}$.

Since $\pi$ is a proof, the infinite branch $\set{\lnsg_i}_{i \in \mathbb{N}}$ must have a suffix $\lnspath= \set{\lnsg_i}_{i \geq j}$ that is a progressing path. Hence, there exists a progressing trace $\set{\tau_i}_{i \geq j}$ along $\lnspath$. Consider the infinite sequence of natural numbers $\set{\mu_i(\tau_i)}_{i\geq j}$. By (3)-(b) and (3)-(c) we have that for each $i \geq j$, $\mu_{i+1}(\tau_{i+1}) \leq \mu_i(\tau_i)$. Since the trace is progressing, there are infinitely many progressing trace pairs $(\tau_i, \tau_{i+1})$, so (3)-(c) implies that there are infinitely many $i \geq j$ with $\mu_{i+1}(\tau_{i+1}) < \mu_i(\tau_i)$. Therefore, $(\mu_i(\tau_i))_i$ is a decreasing sequence of natural numbers that strictly decreases infinitely often. This contradicts the well-foundedness of the natural numbers. Hence, $\lnsg$ must be valid. 
\end{proof}

In our completeness proof below, we proceed by contraposition: given an unprovable LNS $\lnsg$, we show how to extract a counter-model from failed proof-search. 

\begin{customthm}{\ref{thm:completeness-non-wf}}
If $\lnsg$ is valid, then $\calci \proves \lnsg$.
%If $A$ is valid, then $\sar A$ has an end-active proof in $\calci$ with the saturation recurrence property.
\end{customthm}

\begin{proof} We prove the contrapositive and assume that $\lnsg$ does not have a non-wellfounded proof in $\calci$. Let us apply rules from $\calc$ bottom-up to $\lnsg$ in a fair and exhaustive manner, giving rise to a potentially infinite derivation $\der$. Since $\der$ cannot be a proof, it either contains a finite branch ending in a leaf that is not an instance of $\mathsf{id}$ or of $\mathsf{\bot L}$, or by König's lemma, $\der$ contains an infinite branch $\branch := \set{\lnsg_{i}}_{i \in \mathbb{N}}$ which is not progressing. Let us consider the second case. The first case is similar. 

Let $\branch := \set{\lnsg_{i}}_{i \in \mathbb{N}}$ be an infinite branch of $\der$ which is \emph{not} progressing. We use the branch $\branch$ to construct a state sequence $\sts$ such that $\sts \not\sat \lnsg$. Let us define:
$$
\Gamma_{i} := \!\!\!\!\!\!\!\!\!\!\!\!\!\!\!\! \bigcup_{j \in \mathbb{N}, \lnsg_{j}(i) = \Gamma \sar \Delta} \!\!\!\!\!\!\!\!\!\!\!\!\!\!\!\! \Gamma
\qquad
\Delta_{i} := \!\!\!\!\!\!\!\!\!\!\!\!\!\!\!\! \bigcup_{j \in \mathbb{N}, \lnsg_{j}(i) = \Gamma \sar \Delta} \!\!\!\!\!\!\!\!\!\!\!\!\!\!\!\! \Delta
$$
We define $\sigma_{i} = \set{p \mid p \in \Gamma_{i}}$ and $\bar\sigma=\tuple{\sigma_0,\sigma_1,\ldots}$. We now prove the following by a mutual induction on the length of $A$: (1) if $A \in \Gamma_{i}$, then $\sts, i \sat A$ and (2) if $A \in \Delta_{i}$, then $\sts, i \not\sat A$. We show a select number of cases and remark that all remaining cases are similar.
\begin{description}

\item[$A = p \in \Gamma_{i}$.] By definition $p \in \sigma_{i}$, therefore $\sts, i \sat p$.

\item[$A = p \in \Delta_{i}$.] Suppose that $p \in \Delta_{i}$. Assume, for a contradiction, that $p \in \Gamma_{i}$ as well. Then, there would exist a $j$ such that $p \in \Sigma \cap \Pi$ with $\lnsg_{j}(i) = \Sigma \sar \Pi$. Therefore, $\lnsg$ is an instance of $\id$, meaning, $\branch$ must be finite because $\id$ would be applied at some point. This gives a contradiction, and so, $p \not\in \Gamma_{i}$, meaning, $\sts, i \not\sat p$.

\item[$A = \X B \in \Gamma_{i}$.] By our assumption, there exists a $j$ such that $\X B \in \Sigma$ with $\lnsg_{j}(i) = \Sigma \sar \Pi$. Since rules are applied fairly and exhaustively in $\der$, we know that either $\nextli$ or $\nextlii$ will be applied along $\branch$ with $\X B$ principal. Therefore, for some $k \geq j$, $B \in \Sigma'$ with $\lnsg_{k}(i+1) = \Sigma' \sar \Pi'$, implying that $B \in \Gamma_{i+1}$. By IH, it follows that $\sts, i+1 \sat B$, meaning, $\sts, i \sat \X B$.

%\item[$A = \X B \in \Delta_{i}$.] \textcolor{red}{TODO}

\item[$A = B \until C \in \Gamma_{i}$.] By our assumption, there exists a $j$ such that $B \until C \in \Sigma$ with $\lnsg_{j}(i) = \Sigma \sar \Pi$. Since rules are applied fairly and exhaustively in $\der$ and $\branch$ is not progressing, we know that $\untilli$ and $\untillii$ will be applied $k \geq 1$ times above $\lnsg_{j}$ in the branch $\branch$ such that (1) $B \until C$ is principal, (2) for $k-1$ applications, the branch $\branch$ goes through the right premise of $\untilli$ or $\untillii$, and (3) for the $k^\text{th}$ application, the branch $\branch$ goes through the left premise of $\untilli$ or $\untillii$. Therefore, for $0 \leq n < k$, we have $B \in \Gamma_{i+n}$ and $C \in \Gamma_{i+k}$. By IH, $\sts, i+n \sat B$ and $\sts, i+k \sat C$, which implies that $\sts, i \sat B \until C$.

\item[$A = B \until C \in \Delta_{i}$.] By our assumption, there exists a $j$ such that $B \until C \in \Pi$ with $\lnsg_{j}(i) = \Sigma \sar \Pi$. There are two cases to consider. First, it could be the case that $\untilri$ and $\untilrii$ are applied infinitely often above $\lnsg_{j}$ along $\branch$ with $B \until C$ principal and with $\branch$ always going through the right premise of $\untilri$ or $\untilrii$. In this case, we have that $C \in \Delta_{k}$ for all $k \geq i$. By IH, we have that $\sts, k \not\sat C$ for all $k \geq i$, meaning, $\sts, i \not\sat B \until C$. Second, it could be the case that $\untilri$ and $\untilrii$ are applied $k \geq 1$ times above $\lnsg_{j}$ in the branch $\branch$ such that $B \until C$ is principal, the branch $\branch$ goes through the right premise of $\untilri$ or $\untilrii$ for $k-1$ applications, and the branch $\branch$ goes through the left premise of $\untilri$ or $\untilrii$ for the $k^\text{th}$ application. Therefore, for $0 \leq n < k$, we have $C \in \Delta_{i+n}$ and $B,C \in \Delta_{i+k}$. By IH, $\sts, i+n \not\sat C$, $\sts, i+k \not\sat B$, and $\sts, i+k \not\sat C$, which implies that $\sts, i \not\sat B \until C$.

\end{description}
Let $\lnsg(i) = \Sigma_{i} \sar \Pi_{i}$ for $1 \leq i \leq \size{\lnsg}$. As $\Sigma_{i} \subseteq \Gamma_{i}$ and $\Pi_{i} \subseteq \Delta_{i}$ for $1 \leq i \leq \size{\lnsg}$, it follows that $\sts \not\sat \lnsg$.
\end{proof}
