# Supplementary material for: Non-Wellfounded and Cyclic Proofs for LTL: A Syntactic Correspondence with Linear Nested Sequents
Source: arXiv:2606.03413 source file (2026-10-05)
Supplement: Supplementary file 2 [file completeness-appendix.tex]

We prove completeness of $\calci$. We begin by defining proof-search trees and showing that they satisfy the SRP. Then, we show that every LNS $\lnsg$ has a proof-search tree from which either a proof of $\lnsg$ can be extracted or from which a counter-model for $\lnsg$ can be constructed.

We introduce two new inference rules that will be used in the completeness proof for $\calc$. These are taken to be \emph{disjunctive rules} (cf.\cite{Min00,LyoTah26}), meaning, the conclusion is provable whenever at least one premise is provable. By contrast, we refer to the remaining rules in $\calc$ as \emph{conjunctive rules}: the conclusion is provable whenever all premises are provable. Our proof-search tree will consist of both conjunctive and disjunctive rule applications, serving as a "macro-structure" from which we can extract either proofs or counter-models (cf.~\cite{LyoTah26,Lyo26}).


The \emph{focused branching rule} $\fbr$ is shown below and must satisfy conditions (1)-(5). In essence, this rule takes an unfocused LNS as the conclusion, and via a bottom-up application, focuses all formulae of the form $A \until B$ in antecedents of components in all possible ways (as well as copying the conclusion as a premise). Let $\lnsg = \Gamma_{0} \sar \Delta_{0} \sep \cdots \sep \Gamma_{n} \sar \Delta_{n}$ and define the multiset $U(\lnsg) := \set{A \until B \mid \exists 0 \leq i < \size{\lnsg}. A \until B \in \Gamma_{i}}$.
\begin{center}
\AxiomC{$\lnsg_{1} \ \ldots \ \lnsg_{k}$}
\RightLabel{$\fbr$}
\UnaryInfC{$\lnsg$} %$$\Gamma_{0}, A_{0,0} \until B_{0,0}, \ldots, A_{0,n_{0}} \until B_{0,n_{0}} \sar \Delta_{0} \sep \ldots \sep \Gamma_{k}, A_{k,0} \until B_{k,0}, \ldots, A_{k,n_{k}} \until B_{k,n_{k}} \sar \Delta_{k}$}
\DisplayProof
\end{center}

\begin{itemize}

\item[(1)] Each until-formula in $U(\lnsg)$ is unfocused;

\item[(2)] There exists exactly one premise $\lnsg_{1}$ equal to the conclusion;

\item[(3)] Each premise, except $\lnsg_{1}$, contains exactly one occurrence of a formula $A \until B \in U(\lnsg)$ in focus;

\item[(4)] No two premises contain the same occurrence of a formula $A \until B \in U(\lnsg)$ in focus;

\item[(5)] $\set{\lnsg_{1}, \ldots, \lnsg_{k}}$ is the smallest set of LNSs satisfying (2)-(4).

\end{itemize}
The \emph{unfocused branching rule} $\ubr$ is shown below and takes an LNS in focus, and via a bottom-up application, returns one premise with the formula unfocused and another premise identical to the conclusion.
\begin{center}
\AxiomC{$\lnsg \sep \Gamma, A \until B^{\annou} \sar \Delta \sep \lnsh$}
\AxiomC{$\lnsg \sep \Gamma, A \until B^{\annof} \sar \Delta \sep \lnsh$}
\RightLabel{$\ubr$}
\BinaryInfC{$\lnsg \sep \Gamma, A \until B^{\annof} \sar \Delta \sep \lnsh$}
\DisplayProof
\end{center}
We define a \emph{pseudo-derivation} to be a derivation in the calculus $\pcalc := (\calc \setminus \set{\annou,\annof}) \cup \set{\fbr,\ubr}$. %We define an \emph{amenable} branch $\branch$ in a pseudo-derivation $\der$ to be an infinite branch such that (1) no trace is focused and (2) some trace is progressing; otherwise, we call the branch $\branch$ \emph{non-amenable}. Our completeness proof will build a pseudo-derivation of an unprovable nested sequent and use it to extract a counter-model. 
Last, we define the \emph{trivial rule} $\mathsf{triv}$ to be the rule of the form:
\begin{center}
\AxiomC{$\lnsg$}
\RightLabel{$\mathsf{triv}$}
\UnaryInfC{$\lnsg$}
\DisplayProof
\end{center}
Observe that if a trivial rule application occurs in a proof, then it can be `contracted' to a single copy of $\lnsg$, showing its admissibility in $\calc$.

Let us call $\nextlii$, $\nextrii$, $\untillii$ and $\untilrii$ \emph{expansion} rules and all other rules in $\pcalc$ \emph{length-preserving}. An LNS $\lnsg$ is called \emph{fully saturated} \iffi for $0 \leq i < \size{\lnsg}$, $\lnsg$ is $i$-saturated, i.e., $\lnsg$ is not the conclusion of any instance of a rule in $\calci$. We formalize proof-search by means of \emph{proof-search trees} which represent a systematic search for a proof of a given LNS. 

\begin{definition}\label{def:proof-search-tree} A \emph{proof-search tree} for an LNS $\lnsg$ is a pseudo-derivation $\prf$ of $\lnsg$ such that the following hold:
\begin{enumerate}

\item[$(1)$] Every rule instance in $\pi$ is succinct;

\item[$(2)$] The conclusion of every instance of an expansion rule is saturated;

\item[$(3)$] The $\ubr$ and $\fbr$ rules are applied infinitely often along every infinite branch;

\item[$(4)$] Every leaf of $\pi$ is an initial sequent or a fully saturated sequent.

\end{enumerate}
\end{definition}


Intuitively, given an LNS $\lnsg$, we obtain a proof-search tree by applying length-preserving rules bottom-up until every leaf is either an initial sequent or saturated. Branches ending in initial sequents or fully saturated leaves are closed, while branches ending in saturated leaves that are \emph{not fully saturated} are extended by applying a disjunctive rule ($\fbr$ or $\ubr$) bottom-up (depending on if the leaf contains no formula in focus or some formula in focus, resp.), followed by a bottom-up application of an expansion rule. Since the premise of an expansion rule may no longer be saturated, this process can be repeated. We thus obtain the following lemma, whose proof is standard and omitted.


\begin{lemma}
    Every LNS $\lnsg$ has a proof-search tree.
\end{lemma}


The \emph{length} $\lgth{A}$ of a formula $A$ is defined to be the number of symbols it contains. We define $\lgth{A^{\an}} := \lgth{A}$ for $A \in \lang$ and $\an \in \set{\annou,\annof}$. For a set $\Gamma$ of annotated formulae we define $\lgth{\Gamma} := \sum_{A^\an \in \Gamma} \lgth{A^\an}$. Given a Gentzen sequent $\Gamma \sar \Delta$, we define the \emph{size} of $\Gamma \sar \Delta$ to be $s(\Gamma \sar \Delta) := \lgth{\Gamma} + \lgth{\Delta}$. For an LNS $\lnsg = \Gamma_0 \sar \Delta_0 \sep \cdots \sep \Gamma_n \sar \Delta_n$ we define the \emph{size} of $\lnsg$ to be $s(\lnsg) := \sum_{0 \leq i \leq n} s(\Gamma_i \sar \Delta_i)$. A \emph{potential trace value} of $\lnsg$ is a tuple $\tau=\langle A \until B^{\an}, i\rangle$ such that $A \until B^{\an} \in \sufo{\Gamma_i \sar \Delta_i}$ where $\Gamma_i \sar \Delta_i$ is the $i$-component of $\lnsg$. Given a potential trace value $\tau= \langle A \until B^{\an}, i \rangle$ of $\lnsg$, we define its \emph{distance} to be $d(\tau) := \size{\lnsg}-(i+1)$. Let $\mathsf{PTV}_\lnsg$ be the \emph{multiset} of potential trace values of $\lnsg$. Define the \emph{distance} of $\lnsg$ to be $d(\lnsg) := \sum_{A \until B^{\an} \in \mathsf{PTV}_\lnsg} d(A \until B^{\an})$. For the following lemma we consider the tuple $\langle d(\lnsg), s(\lnsg)\rangle$ where $<_l$ is the standard lexicographical order on $\mathbb{N} \times \mathbb{N}$. It is well-known that $<_l$ is a well-order.

 \begin{lemma}\label{lem: measure decrease} Let $\mathsf{r}$ be a length-preserving rule and consider a succinct instance of $\mathsf{r}$ with conclusion $\lnsg$ and a premise $\lnsh$. Then, $\langle d(\lnsh), s(\lnsh)\rangle <_l \langle d(\lnsg), s(\lnsg)\rangle$.
 \end{lemma}
 \begin{proof}
  Since $\mathsf{r}$ is a length-preserving rule, note that $\size{\lnsg} = \size{\lnsh}$. If $\mathsf{r} \not \in \set{\untilli, \untilri}$, then the claim of the lemma follows immediately from inspection of the rules and the fact that the application of $\mathsf{r}$ is succinct, as in each case $d(\lnsh) \leq d(\lnsg)$ and $s(\lnsh) < s(\lnsg)$. For $\mathsf{r} = \untilli$, if $\lnsh$ is the left premise, the claim immediately follows. If $\lnsh$ is the right premise, then the size of $\lnsh$ may increase, but since the instance is succinct, we have $d(\lnsh) < d(\lnsg)$ and so the claim holds. The case for $\mathsf{r} = \untilri$ is similar.\footnote{Note that it is crucial to use the \emph{multiset} of potential trace values for this argument, since when using the \emph{set} of potential trace values, the measure might not decrease and can even increase in some situations. For example, if we use sets of potential trace values and consider an application of $\untilli$ with conclusion $\lnsg := \Omega \mid \X (p \until q), p \until q^\an \sar \emptyset \sep \X (p \until q) \sar \emptyset$ and right premise $\lnsh := \Omega' \mid \X (p \until q), p \sar \emptyset \sep \X (p \until q), p \until q^\anb \sar \emptyset$, then $\langle d(\lnsg), s(\lnsg) \rangle = \langle 1, 11 \rangle < \langle 1, 12 \rangle = \langle d(\lnsh), s(\lnsh) \rangle$.}
 \end{proof}
 


\begin{lemma}\label{lem: SRP}
    Let $\lnsg$ be an LNS and $\pi$ be a proof-search tree for $\lnsg$. Then, $\pi$ satisfies the SRP.
\end{lemma}
\begin{proof} Suppose, toward a contradiction, that $\pi$ is a proof-search tree for $\lnsg$ which does not satisfy the SRP. Then, there exists an infinite branch $\branch = \set{\lnsg_i}_{i \in \mathbb{N}}$ and $j \in \mathbb{N}$ such that for all natural numbers $i \geq j$ the LNS $\lnsg_i$ is not saturated. By the definition of a proof-search tree the suffix $\lnspath_j=\set{\lnsg_i}_{i \geq j}$ of $\branch$ starting at $\lnsg_j$ only passes through instances of length-preserving rules. Moreover, each such instance is succinct. Therefore, by Lemma~\ref{lem: measure decrease}, $\set{\langle d(\lnsg_i), s(\lnsg_i)\rangle}_{i \geq j}$ is an infinite and strictly decreasing sequence in $<_l$, which contradicts that $<_l$ is a well-order. Hence, $\pi$ satisfies the SRP.
\end{proof}

We claim that along any infinite branch $\branch = \set{\lnsg_i}_{i \in \mathbb{N}}$ of a proof-search tree $\pi$, the length $\size{\lnsg_i}$ grows unboundedly, i.e., there are infinitely many $i \in \mathbb{N}$ such that $\size{\lnsg_i} < \size{\lnsg_{i+1}}$. To see this, observe that since $\pi$ satisfies the SRP, infinitely many $\lnsg_i$ are saturated. After each saturated sequent, the proof-search procedure applies an expansion rule. Although taking the left premise of an expansion rule (e.g., $\untilrii$ or $\untillii$) may yield a premise that is itself saturated without increasing the length, this situation can only repeat finitely many times: since the instance is succinct and each component contains a \emph{finite} set of annotated formulae, every left-premise application strictly decreases the size of the end component. Hence, after finitely many such steps, the branch must pass through an expansion rule whose premise has strictly greater length.


We now define two dual notions of subtree within a proof-search tree. Intuitively, a \emph{CB-structure} represents a potential proof of $\lnsg$, while a \emph{DB-structure} represents a potential counter-model.

\begin{definition}[CB- and DB-Closure]\label{def:CB-DB-closure}
Let $\prf$ be a proof-search tree for $\lnsg$. A \emph{CB-structure} is a subtree $(T, \prec)$ of $\prf$ such that $\lnsg \in T$ and for each $\lnsh \in T$:
\begin{itemize}

\item[$(1)$] If $\lnsh$ is the conclusion of a conjunctive rule, then all premises are in $T$;

\item[$(2)$] If $\lnsh$ is the conclusion of a disjunctive rule, then exactly one premise is in $T$.

\end{itemize}

\noindent
A \emph{DB-structure} is a subtree $(T, \prec)$ of $\prf$ such that $\lnsg \in T$ and for each $\lnsh \in T$:
\begin{itemize}

\item[$(1)$] If $\lnsh$ is the conclusion of a conjunctive rule, then exactly one premise is in $T$;

\item[$(2)$] If $\lnsh$ is the conclusion of a disjunctive rule, then all premises are in $T$.

\end{itemize}

\noindent
The \emph{CB-closure} $\cbclo(\prf)$ is the set of all CB-structures of $\prf$, and the \emph{DB-closure} $\dbclo(\prf)$ is the set of all DB-structures of $\prf$.
\end{definition}

We remark that since a CB-structure selects exactly one premise at each disjunctive node, and since both $\fbr$ and $\ubr$ include a premise identical to the conclusion (see condition (2) of $\fbr$ and the right premise of $\ubr$), a CB-structure may contain instances of $\mathsf{triv}$. As noted above, such instances are admissible and can be eliminated by contracting the premise and conclusion into a single node. For the remaining (non-trivial) instances, a pruned $\fbr$ application reduces to an instance of $\annof$ (focusing a single formula), and a pruned $\ubr$ application reduces to an instance of $\annou$ (unfocusing a formula). We therefore assume without loss of generality that all instances of $\mathsf{triv}$ have been removed from CB-structures, and identify the remaining pruned $\fbr$ and $\ubr$ applications with $\annof$ and $\annou$ instances, respectively.

A branch in a proof-search tree is \emph{successful} if it either terminates at an initial sequent or is infinite and progressing; it is \emph{failed} if it either terminates at a fully saturated sequent or is infinite and not progressing. Note that every branch is either successful or failed (but not both), since by Definition~\ref{def:proof-search-tree}--(4), every finite branch terminates at either an initial or fully saturated sequent.


\begin{lemma}\label{lem:DB-CB-dual}
Let $\prf$ be a proof-search tree for $\lnsg$. Then, $\cbclo(\prf)$ contains an $\calci$-proof \iffi every DB-structure in $\dbclo(\prf)$ contains a successful branch.
\end{lemma}

\begin{proof}
We interpret the proof-search tree $\prf$ as the arena of a two-player game between \emph{Prover} and \emph{Refuter}:
\begin{itemize}

\item At conjunctive (binary) nodes, Refuter chooses a premise;

\item At disjunctive ($\fbr$ or $\ubr$) nodes, Prover chooses a premise;

\item At unary nodes, the move is forced.

\end{itemize}
A \emph{play} is a maximal path through $\prf$ determined by the players' choices. Prover wins a play if it is successful; Refuter wins otherwise. We observe the following correspondence between strategies and closures:
\begin{itemize}

\item A \emph{Prover strategy} determines a CB-structure: at disjunctive nodes, one premise is retained (Prover's choice), while at conjunctive nodes, both premises are retained. A Prover strategy is \emph{winning} \iffi the corresponding CB-structure is a proof.

\item A \emph{Refuter strategy} determines a DB-structure: at conjunctive nodes, one premise is retained (Refuter's choice), while at disjunctive nodes, all premises are retained. A Refuter strategy is \emph{winning} \iffi the corresponding DB-structure has no successful branch.

\end{itemize}
Under this correspondence, we obtain:
\begin{align*}
\cbclo(\prf) \text{ contains a proof} \;&\iff\; \text{Prover has a winning strategy} \\
&\iff\; \text{Refuter has no winning strategy} \\
&\iff\; \text{every DB-structure has a successful branch}
\end{align*}
The first equivalence follows from the strategy--structure correspondence: a winning Prover strategy is precisely a CB-structure in which every branch is successful, i.e., a proof. The third equivalence is analogous: a winning Refuter strategy is precisely a DB-structure in which every branch is failed. It remains to justify the second equivalence, which is the determinacy of the game.

The winning condition for Prover is Borel: whether a finite play is successful depends only on the leaf reached (a condition determined by a finite prefix), while whether an infinite play is progressing is determined by countable conditions on the play's steps---specifically, the existence of a starting index from which (i)~every step preserves a formula in focus and (ii)~infinitely many steps pass through the right premise of $\untilli$ or $\untillii$ with that formula principal. Each of these is expressible as a countable intersection or union of conditions depending on finitely many steps of the play. By Martin's Borel Determinacy Theorem~\cite{Mar75}, the game is determined, which completes the proof.
\end{proof}

A \emph{trace value} is a pair $\tri = \bracket{A \until B^{\an}, i}$ where $A \until B \in \lang$, $\an \in \set{\annof, \annou}$, and $i \in \mathbb{N}$. Given a linear nested sequent $\lnsg = \Gamma_{0} \sar \Delta_{0} \sep \cdots \sep \Gamma_{n} \sar \Delta_{n}$, a trace value $\bracket{A \until B^{\an}, i}$ is a \emph{trace value of~$\lnsg$} if $A \until B^{\an} \in \Gamma_i$ for some $0 \leq i \leq n$. Let $\ru$ be a rule with conclusion $\lnsg$ and premise $\lnsh$. A pair $(\bracket{A \until B^{\an}, i},\, \bracket{A \until B^{\an}, j})$ is a \emph{trace pair} for $(\lnsg, \lnsh)$ \iffi $\bracket{A \until B^{\an}, i}$ is a trace value of $\lnsg$, $\bracket{A \until B^{\an}, j}$ is a trace value of $\lnsh$, and one of the following holds:
%
\begin{enumerate}
\item[$(1)$] $A \until B^{\an}$ is not principal in $\ru$ and $j = i$; or
\item[$(2)$] $A \until B^{\an}$ is principal in $\ru \in \set{\untilli, \untillii}$, $\lnsh$ is the right premise of $\ru$, and $j = i + 1$.
\end{enumerate}
%
A trace pair is \emph{progressing} if $j = i + 1$. A \emph{trace} along a path $\lnspath = \set{\lnsg_{i}}_{i \in \idxset}$ is a sequence of trace values $\set{\tau_{i}}_{i \in \idxset}$ such that $(\tau_i, \tau_{i+1})$ is a trace pair for $(\lnsg_{i}, \lnsg_{i{+}1})$ for each $i$. A trace along an infinite path is \emph{strongly progressing} if infinitely many of its trace pairs are progressing. An infinite path is \emph{strongly progressing} if it admits a strongly progressing trace, and an infinite branch is \emph{strongly progressing} if it contains a suffix that is a strongly progressing path.



\begin{lemma}\label{lem:no-prog-no-strongly-prog}
Let $\prf$ be a proof-search tree. If a DB-structure in $\dbclo(\prf)$ does not contain a progressing branch, then it contains a branch that is not strongly progressing.
\end{lemma}

\begin{proof}
Let $\alpha \in \dbclo(\prf)$ be a DB-structure without a progressing branch. We construct a branch $\branch = \set{\lnsg_i}_{i \in I}$ in $\alpha$ that is not strongly progressing. Set $\lnsg_0 := \lnsg$ (the root of $\prf$). If at any point during the construction, $\branch$ reaches a fully saturated leaf, then $\branch$ is finite and hence trivially not strongly progressing, so we are done. Otherwise, we define $\branch$ as an infinite branch by specifying our choices at $\fbr$ and $\ubr$ nodes as follows:
\begin{itemize}

\item \textit{At $\fbr$ nodes:} Select the premise that puts in focus the until-formula $A \until B \in U(\lnsg_i)$ whose trace along $\branch$ started earliest, i.e., the formula that has been continuously present in some antecedent for the longest stretch going back toward $\lnsg_0$. Ties are broken using a fixed total order on $\sufo{\lnsg}$.

\item \textit{At $\ubr$ nodes:} Select the premise that keeps the current formula in focus (the right premise).

\end{itemize}
At all other nodes, the successor is uniquely determined: by the rule at unary nodes, and by $\alpha$'s choice at binary (conjunctive) nodes.

We claim that $\branch$ is not strongly progressing. Suppose for contradiction that $\branch$ admits a strongly progressing trace $\tau = \set{\tau_k}_{k \geq m}$ for some formula $A \until B$. Since $\tau$ progresses infinitely often, it never terminates (i.e., $A \until B$ remains active along an infinite suffix of $\branch$). We derive a contradiction from two statements:

\medskip
\noindent
\textit{Step 1: Focused traces terminate.} We show that if a formula $C \until D^{\annof}$ is focused at some point along $\branch$ and kept in focus (by choosing the right premise at every subsequent $\ubr$), then the trace of $C \until D$ must eventually terminate. Suppose not. Then after $C \until D$ is focused, the proof-search tree applies $\untilli$ or $\untillii$ with $C \until D^{\annof}$ principal infinitely often (by the proof-search procedure), and since the trace does not terminate, $\alpha$ must choose the right premise at each such application, causing the trace to progress infinitely. But then $\branch$ has a suffix with:
\begin{itemize}
\item[(i)] a continuous focus trace (since $C \until D^{\annof}$ remains in focus), and
\item[(ii)] infinitely many passages through the right premise of $\untilli$ or $\untillii$ with $C \until D^{\annof}$ principal.
\end{itemize}
This makes $\branch$ a progressing branch of $\alpha$, contradicting our assumption.

\medskip
\noindent
\textit{Step 2: Every persistent trace is eventually focused.} Consider the strongly progressing trace $\tau$ for $A \until B$ starting at index $j_0$. At each $\fbr$ node after $j_0$ where $A \until B \in U(\lnsg_i)$, our strategy focuses the earliest-starting active trace. If $\tau$ is not the earliest at a given $\fbr$, then some trace $\sigma$ that started at an index ${<}\, j_0$ is focused instead. By Step~1, $\sigma$'s trace terminates. Since $\sufo{\lnsg}$ is finite and only finitely many components exist at any point before $j_0$, there are only finitely many traces that started before $\tau$. After finitely many $\fbr$ applications---each eliminating the current earliest trace---$\tau$ becomes the earliest-starting active trace and is focused at the next $\fbr$.

\medskip
\noindent
\textit{Contradiction.} By Step~2, $\tau$ is eventually focused. By Step~1, once focused, $\tau$'s trace terminates. But $\tau$ was assumed to progress infinitely often, and a terminated trace cannot progress further. This is a contradiction. Therefore, no trace along $\branch$ progresses infinitely often, meaning $\branch$ is not strongly progressing.
\end{proof}


We now show that every LNS either has an $\calci$-proof satisfying the SRP or is falsifiable, from which completeness follows immediately.

\begin{lemma}\label{lem: proof or falsifiable} Let $\lnsg$ be an LNS. Then, either $\lnsg$ has an $\calci$-proof satisfying the SRP or there exists a state sequence $\Bar{\sigma}$ such that $\Bar{\sigma} \not \sat \lnsg$.
\end{lemma}

\begin{proof} Let $\lnsg$ be an LNS and let $\pi$ be a proof-search tree for $\lnsg$. If $\cbclo(\prf)$ contains an $\calci$-proof of $\lnsg$, then it satisfies the SRP by Lemma~\ref{lem: SRP}. Suppose otherwise that $\cbclo(\prf)$ does not contain an $\calci$-proof. By Lemma~\ref{lem:DB-CB-dual}, some DB-structure $\alpha$ in $\dbclo(\prf)$ contains only failed branches. In particular, $\alpha$ contains no progressing branch, so by Lemma~\ref{lem:no-prog-no-strongly-prog}, $\alpha$ contains a branch $\branch$ that is not strongly progressing. Either $\branch$ is finite (ending in a fully saturated sequent) or infinite and not strongly progressing. We treat only the latter case, as the former is argued similarly. Let $\branch := \set{\lnsg_{i}}_{i \in \mathbb{N}}$ be an infinite branch of $\alpha$ that is \emph{not} strongly progressing.

We use $\branch$ to construct a state sequence $\sts$ such that $\sts \not\sat \lnsg$. Define:
$$
\Gamma_{i} := \!\!\!\!\!\!\!\!\!\!\!\!\!\!\!\! \bigcup_{j \in \mathbb{N}, \, \lnsg_{j}(i) \, = \, (\Gamma \, \sar \, \Delta)} \!\!\!\!\!\!\!\!\!\!\!\!\!\!\!\! \Gamma^{-}
\qquad
\Delta_{i} := \!\!\!\!\!\!\!\!\!\!\!\!\!\!\!\! \bigcup_{j \in \mathbb{N}, \, \lnsg_{j}(i) \, = \, (\Gamma \, \sar \, \Delta)} \!\!\!\!\!\!\!\!\!\!\!\!\!\!\!\! \Delta^{-}
$$
That is, $\Gamma_i$ collects all unannotated formulae appearing in the antecedent of the $i$-component along $\branch$, and $\Delta_i$ collects those in the consequent. We define $\sigma_{i} := \set{p \mid p \in \Gamma_{i}}$ and $\bar\sigma := \tuple{\sigma_0,\sigma_1,\ldots}$. We prove the following by mutual induction on the length of $A$:
\begin{enumerate}
\item[(1)] If $A \in \Gamma_{i}$, then $\sts, i \sat A$;
\item[(2)] If $A \in \Delta_{i}$, then $\sts, i \not\sat A$.
\end{enumerate}

\case{Case $A = \bot \in \Gamma_i$.} There exists $j$ such that $\bot \in \lnsg_j(i)$, making $\lnsg_j$ an initial sequent. By Definition~\ref{def:proof-search-tree}-(4), the branch $\branch$ terminates at $\lnsg_j$, contradicting the assumption that $\branch$ is infinite. Hence $\bot \not \in \Gamma_i$.

\case{Case $A = \bot \in \Delta_i$.} By definition, $\sts, i \not \models \bot$.

\case{Case $A = p \in \Gamma_{i}$.} By definition, $p \in \sigma_{i}$, so $\sts, i \sat p$.

\case{Case $A = p \in \Delta_{i}$.} Suppose for contradiction that $p \in \Gamma_{i}$ as well. Then there exist $j_0, j_1$ with $\lnsg_{j_0}(i) = \Sigma \sar \Pi$ and $\lnsg_{j_1}(i) = \Sigma' \sar \Pi'$ such that $p \in \Sigma$ and $p \in \Pi'$. Without loss of generality, assume $j_0 \leq j_1$. Since no rule in $\calci$ deletes atoms, $p \in \Sigma$ implies $p \in \Sigma'$. Therefore $p \in \Sigma' \cap \Pi'$, making $\lnsg_{j_1}$ an instance of $\id$. By Definition~\ref{def:proof-search-tree}-(4), the branch $\branch$ terminates at $\lnsg_{j_1}$, contradicting our assumption. Hence $p \not\in \Gamma_{i}$, and so $\sts, i \not \sat p$.

\case{Case $A = B \to C \in \Delta_i$.} There exists $j$ such that $B \to C \in \Pi$ with $\lnsg_j(i) = \Sigma \sar \Pi$. Since $\pi$ satisfies the SRP, there exists $k > j$ such that $\lnsg_k$ is saturated and $\size{\lnsg_{j}} < \size{\lnsg_{k}}$. The latter implies that an expansion rule was applied between $\lnsg_j$ and $\lnsg_k$, which forces $B \to C$ to be decomposed by ${\to}\mathsf{R}$ in the segment of $\branch$ between $\lnsg_j$ and $\lnsg_k$. Hence, for some $j \leq l \leq k$ with $\lnsg_l(i) = \Sigma' \sar \Pi'$, we have $B \in \Sigma'$ and $C \in \Pi'$, giving $B \in \Gamma_i$ and $C \in \Delta_i$. By IH, $\Bar{\sigma}, i \sat B$ and $\Bar{\sigma}, i \not \sat C$, so $\Bar{\sigma}, i \not \sat B \to C$. The case for $A = B \to C \in \Gamma_i$ is similar and omitted.

\case{Case $A = \X B \in \Gamma_{i}$.} There exists $j$ such that $\X B \in \Sigma$ with $\lnsg_{j}(i) = \Sigma \sar \Pi$. Since $\pi$ satisfies the SRP, there exists $k > j$ such that $\lnsg_k$ is saturated and $\size{\lnsg_{j}} < \size{\lnsg_{k}}$. By the same reasoning as above, $\X B$ must be decomposed by $\nextli$ or $\nextlii$ in the segment between $\lnsg_j$ and $\lnsg_k$. Hence, for some $j \leq l \leq k$ with $\lnsg_l(i+1) = \Sigma' \sar \Pi'$, we have $B \in \Sigma'$, giving $B \in \Gamma_{i+1}$. By IH, $\sts, i+1 \sat B$, and so $\sts, i \sat \X B$. The case for $A = \X B \in \Delta_i$ is similar and omitted.

\case{Case $A = B \until C \in \Gamma_{i}$.} There exists $j$ such that $B \until C^\an \in \Sigma$ with $\lnsg_{j}(i) = \Sigma \sar \Pi$. Since $\pi$ satisfies the SRP, there exists an instance of $\untilli$ or $\untillii$ above $\lnsg_j$ in $\branch$ with $B \until C^\an$ principal. Since $\branch$ is not strongly progressing, $\branch$ cannot pass through the right premise of $\untilli$ or $\untillii$ with $B \until C^\an$ principal infinitely often (as this would yield a strongly progressing trace). Therefore, there exists $k \geq 1$ such that $\untilli$ or $\untillii$ is applied $k$ times above $\lnsg_j$ with $B \until C^\an$ principal, where $\branch$ goes through the right premise for the first $k-1$ applications and through the left premise for the $k^\text{th}$. It follows that $B \in \Gamma_{i+n}$ for $0 \leq n < k-1$ and $C \in \Gamma_{i+k-1}$. By IH, $\sts, i+n \sat B$ and $\sts, i+k-1 \sat C$, which gives $\sts, i \sat B \until C$.

\case{Case $A = B \until C \in \Delta_{i}$.} There exists a $j$ such that $B \until C \in \Pi$ with $\lnsg_{j}(i) = \Sigma \sar \Pi$. We distinguish two sub-cases:

\emph{Sub-case 1:} $\untilri$ or $\untilrii$ is applied infinitely often above $\lnsg_{j}$ along $\branch$ with $B \until C$ principal and $\branch$ always going through the right premise. Then $C \in \Delta_{k}$ for all $k \geq i$. By IH, $\sts, k \not\sat C$ for all $k \geq i$, so $\sts, i \not\sat B \until C$.

\emph{Sub-case 2:} There exists $k \geq 1$\footnote{We have $k \geq 1$ since the SRP guarantees that between $\lnsg_j$ and the next saturated sequent of strictly greater length, the formula $B \until C$ is decomposed at least once by $\untilri$ or $\untilrii$.} such that $\untilri$ or $\untilrii$ is applied $k$ times above $\lnsg_{j}$ with $B \until C$ principal, where $\branch$ goes through the right premise for the first $k-1$ applications and through the left premise for the $k^\text{th}$. Then $C \in \Delta_{i+n}$ for $0 \leq n < k-1$ and $B, C \in \Delta_{i+k-1}$. By IH, $\sts, i+n \not\sat C$, $\sts, i+k-1 \not\sat B$, and $\sts, i+k-1 \not\sat C$, which gives $\sts, i \not\sat B \until C$.

\medskip
\noindent
Finally, let $\lnsg(i) = \Sigma_{i} \sar \Pi_{i}$ for $0 \leq i < \size{\lnsg}$. Since $\Sigma_{i}^{-} \subseteq \Gamma_{i}$ and $\Pi_{i}^{-} \subseteq \Delta_{i}$ for each $0 \leq i < \size{\lnsg}$, it follows that $\sts, i \not\sat \lnsg(i)$ for all $0 \leq i < \size{\lnsg}$. Hence, by Definition~\ref{def: satisfaction LNS}, $\Bar{\sigma} \not \sat \lnsg$.
\end{proof}


\begin{customthm}{\ref{thm:completeness-non-wf}}[Completeness of $\calci$] If $\lnsg$ is valid, then $\lnsg$ has an $\calci$-proof satisfying the SRP.
\end{customthm}
\begin{proof} Suppose $\lnsg$ is valid and let $\prf$ be a proof-search tree for $\lnsg$. By Lemma~\ref{lem: proof or falsifiable}, either $\cbclo(\pi)$ contains a proof of $\lnsg$ satisfying the SRP or $\lnsg$ is falsifiable. Since $\lnsg$ is valid, the latter is impossible, so $\cbclo(\pi)$ contains a proof of $\lnsg$ satisfying the SRP.
\end{proof}
