# Supplementary material for: Non-Wellfounded and Cyclic Proofs for LTL: A Syntactic Correspondence with Linear Nested Sequents
Source: arXiv:2606.03413 source file (2026-10-05)
Supplement: Supplementary file 3 [file cyclic-to-nwf-appendix.tex]

We provide the skipped proofs of Section~\ref{subsec:unravel}. In order to prove Lemma~\ref{cor: corresponding paths}, we first prove the following auxiliary lemma.

\begin{lemma}\label{lem: corresponding paths} For any $j \in \mathbb{N}$ and every finite looping path $\lnspath^\circ_{j+1}$ of $(\pi_{j+1}, L_{j+1}, c_{j+1})$, there exists a looping path $\lnspath^\circ_j$ of $(\pi_j, L_j, c_j)$ of equal length, such that $\lnspath^\circ_{j+1}$ corresponds to $\lnspath^\circ_j$.
\end{lemma}

\begin{proof}
Recall that ($\ast$) $(\pi_{j+1}, L_{j+1}, c_{j+1})$ was obtained by `pasting' the cyclic proof $(\pi', L', c')$ above $\lnsh$ in $\pi_j$, where $\lnsh \in L_j$ with $c_j(\lnsh)$ a minimal companion and $(\pi', L', c')$ is strictly isomorphic to the cyclic proof $(\pi, L, c)$ rooted at $c_j(\lnsh)$ in $(\pi_j, L_j, c_j)$, as given by the Shifting Lemma. Let $h \colon \pi \to \pi'$ denote the strict isomorphism.

Let $\lnspath_{j+1}^\circ = \set{\lnsg_i}_{i \leq k}$ be a finite looping path of $(\pi_{j+1}, L_{j+1}, c_{j+1})$. Since $\pi_{j+1}$ was obtained by pasting $\pi'$ above $\lnsh$ in $\pi_j$, there exists a largest natural number $t \leq k$ such that the initial segment $\lnspath^\circ[t] = \set{\lnsg_i}_{i \leq t}$ of $\lnspath^\circ_{j+1}$ is a looping path of $(\pi_j, L_j, c_j)$. If $t = k$, then let $\lnspath^\circ_j := \lnspath^\circ_{j+1}$ and note that $\lnspath^\circ_j$ and $\lnspath^\circ_{j+1}$ are trivially corresponding (they are the same sequence in the same derivation, which is a sub-derivation of~$\pi_{j+1}$). Otherwise, $\lnsg_t = \lnsh$ and the suffix of $\lnspath^\circ_{j+1}$ starting at $\lnsg_t$ is a looping path of $(\pi', L', c')$ by construction. Define
%
\[
\lnspath^\circ_j := \lnspath^\circ[t] \circ \set{h^{-1}(\lnsg_i)}_{t < i \leq k}
\]
%
where $\circ$ denotes sequence concatenation. We verify that $\lnspath^\circ_j$ is a well-defined looping path of $(\pi_j, L_j, c_j)$.

The initial segment $\lnspath^\circ[t]$ ends at the bud $\lnsg_t = \lnsh \in L_j$ with companion $c_j(\lnsh)$. Since $\lnsg_{t+1}$ is a child of $\lnsh$ in $\pi_{j+1}$ (equivalently, a child of the root of $\pi'$) and $h$ maps the root $c_j(\lnsh)$ of $\pi$ to the root $\lnsh$ of $\pi'$, it follows that $h^{-1}(\lnsg_{t+1})$ is a child of $c_j(\lnsh)$ in $\pi_j$, as required by Definition~\ref{dfn:looping-path}--(3). The remainder of the suffix $\set{h^{-1}(\lnsg_i)}_{t < i \leq k}$ is a looping path through $(\pi, L, c)$ since $h^{-1}$ is a homomorphism. Moreover, the suffix is well-defined since $c_j(\lnsh)$ is a minimal companion, ensuring that the subtree of $\pi_j$ rooted at $c_j(\lnsh)$ forms a self-contained cyclic proof. It remains to verify that $\lnspath^\circ_{j+1}$ and $\lnspath^\circ_j$ are corresponding, i.e., that conditions (1)--(4) of Definition~\ref{dfn:corresponds} hold for all $i \leq k$.

\case{Case for $i < t$:} Both paths contain the same LNS $\lnsg_i$ appearing in the same position of the same sub-derivation $\pi_j$ (which is contained in $\pi_{j+1}$). Hence conditions (1)--(4) hold trivially.

\case{Case for $i = t$:} Both paths contain $\lnsg_t = \lnsh$. In $\lnspath^\circ_{j+1}$, the transition from $\lnsg_t$ to $\lnsg_{t+1}$ is governed by the rule applied to $\lnsh$ in $\pi_{j+1}$ (i.e., the root rule of $\pi'$). In $\lnspath^\circ_j$, the transition from $\lnsg_t$ to $h^{-1}(\lnsg_{t+1})$ is a loop jump governed by the rule applied to $c_j(\lnsh)$ in $\pi_j$ (i.e., the root rule of $\pi$). Since $h$ is a strict isomorphism mapping the root rule of $\pi$ to the root rule of $\pi'$, condition (1) holds. Condition (2) holds as well: if $\lnsg_{t+1}$ is the right (resp.\ left) premise of the root rule of $\pi'$, then $h^{-1}(\lnsg_{t+1})$ is the right (resp.\ left) premise of the root rule of $\pi$, since $h$ preserves parent-child relationships and premise positions. For condition (3): since both paths contain the same LNS $\lnsg_t = \lnsh$ at position $t$, the LNS trivially has the same focus status. Moreover, by invariant (I)(c) of the Shifting Lemma, since $c_j(\lnsh)$ is saturated and all rule applications occur at components with index $\geq n$, the annotations (and thus focus) on the principal formula of the root rule of $\pi$ are identical to those of the root rule of $\pi'$. Hence, if the principal formula of the rule applied to $\lnsg_t$ in $\lnspath^\circ_{j+1}$ is in focus, then the principal formula of the rule applied to $\lnsg_t$ in $\lnspath^\circ_j$ is in focus (and vice versa). For condition (4): $\lnsg_t = \lnsh$ is saturated in both paths (by the definition of cyclic proofs, both $\lnsh$ and $c_j(\lnsh)$ are saturated), and $\last{\lnsg_t}$ is the same in both paths since both contain the same LNS $\lnsh$.

\case{Case for $t < i \leq k$:} In $\lnspath^\circ_{j+1}$, the LNS at index $i$ is $\lnsg_i$ (in $\pi'$), while in $\lnspath^\circ_j$, the LNS at index $i$ is $h^{-1}(\lnsg_i)$ (in $\pi$). Since both $h$ and $h^{-1}$ are homomorphisms, condition (1) holds: $\lnsg_i$ is the conclusion of an instance of rule $\mathsf{r}$ in $\pi'$ if and only if $h^{-1}(\lnsg_i)$ is the conclusion of an instance of $\mathsf{r}$ in $\pi$. Condition (2) holds similarly: homomorphisms preserve parent-child relationships, so the same premise (left or right) is selected. For condition (3): by invariant (I)(c) of the Shifting Lemma, for components at index $i \geq n$, we have $\lnsf(i) = h(\lnsf)(j)$ with $j = k + (i-n)$. Since $c_j(\lnsh)$ is saturated, all rule applications occur at components with index $\geq n$, and these components are preserved (only shifted in position) by $h$. In particular, the annotations are identical, so $\lnsg_i$ contains a formula in focus if and only if $h^{-1}(\lnsg_i)$ contains a formula in focus. Moreover, if the principal formula of the rule applied to $\lnsg_i$ is in focus, then the principal formula of the corresponding rule applied to $h^{-1}(\lnsg_i)$ is in focus (and vice versa), since the annotation on the principal formula is preserved by $h$. For condition (4): by invariant (I), $\lnsg_i$ is saturated if and only if $h^{-1}(\lnsg_i)$ is saturated, and if so, $\last{h^{-1}(\lnsg_i)} = \last{\lnsg_i}$.

Therefore, $\lnspath^\circ_{j+1}$ and $\lnspath^\circ_j$ are corresponding.
\end{proof}


\begin{customlem}{\ref{cor: corresponding paths}} For any $j \in \mathbb{N}$ and every finite looping path $\lnspath^\circ_j$ of $(\pi_{j}, L_{j}, c_{j})$, there exists a finite looping path $\lnspath^\circ_0$ of $(\pi_0, L_0, c_0)$ of equal length, such that $\lnspath^\circ_j$ and $\lnspath^\circ_0$ are corresponding.
\end{customlem}

\begin{proof} By induction on $j$. The base case for $j = 0$ is trivial. Thus, suppose $j = n+1$ and consider a finite looping path $\lnspath^\circ_{n+1}$ of $(\pi_{n+1}, L_{n+1}, c_{n+1})$. By Lemma~\ref{lem: corresponding paths}, there exists a finite looping path $\lnspath^\circ_n$ of $(\pi_n, L_n, c_n)$ of equal length, such that $\lnspath^\circ_{n+1}$ and $\lnspath^\circ_n$ are corresponding. By the induction hypothesis, there exists a finite looping path $\lnspath^\circ_0$ of $(\pi_0, L_0, c_0)$ of equal length, such that $\lnspath^\circ_n$ and $\lnspath^\circ_0$ are corresponding. Since the notion of correspondence between looping paths is transitive (each condition is a biconditional that composes), $\lnspath^\circ_{n+1}$ and $\lnspath^\circ_0$ are corresponding as well.
\end{proof}
